# Supplementary material for: Interfacial and bulk switching MoS2 memristors for an all-2D reservoir computing framework
Source: arXiv:2511.16557 source file (2025-11-20)
Supplement: Supplementary file 1 [file RC_computing_MoS2_v4_supplementary.pdf]

# Interfacial and bulk switching MoS<sub>2</sub> memristors for an all-2D reservoir computing framework

Asmita S. Thool,<sup>†</sup> Sourodeep Roy,<sup>†</sup> Prahalad Kanti Barman,<sup>‡</sup> Kartick Biswas,<sup>¶</sup>  
Pavan Nukala,<sup>¶</sup> Abhishek Misra,<sup>‡</sup> Saptarshi Das,<sup>§</sup> and Bhaswar Chakrabarti<sup>\*,†</sup>

<sup>†</sup>*Department of Electrical Engineering, Indian Institute of Technology Madras, India*

<sup>‡</sup>*Department of Physics, Indian Institute of Technology Madras, India*

<sup>¶</sup>*Center for Nano Science and Engineering, Indian Institute of Science, Bangalore, India*

<sup>§</sup>*The Pennsylvania State University, University Park, PA, USA*

E-mail: bchakrabarti@ee.iitm.ac.in, sud70@psu.edu

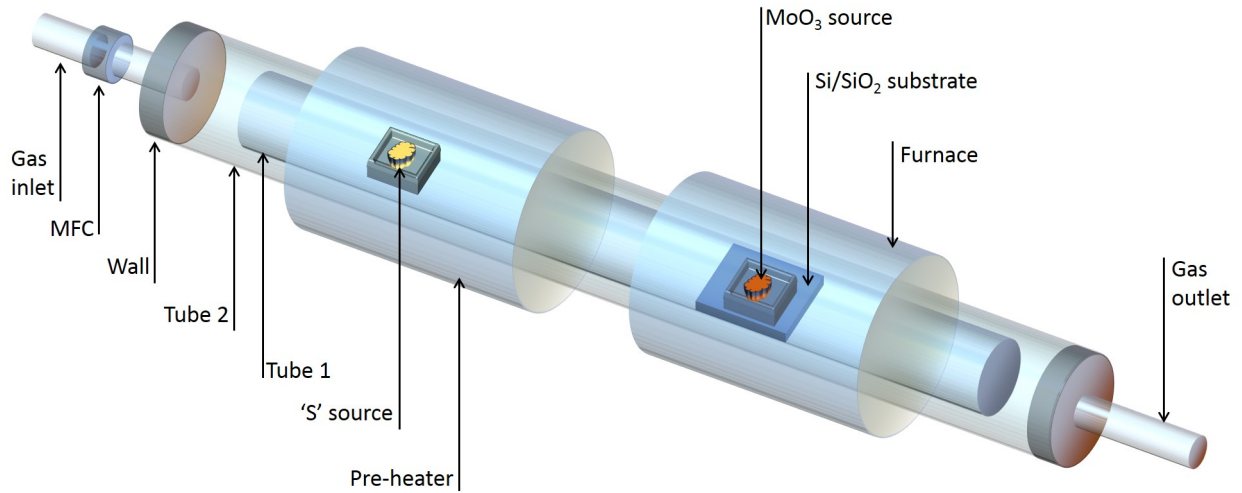

Figure S1 – Schematic diagram of Chemical Vapor Deposition (CVD) system.

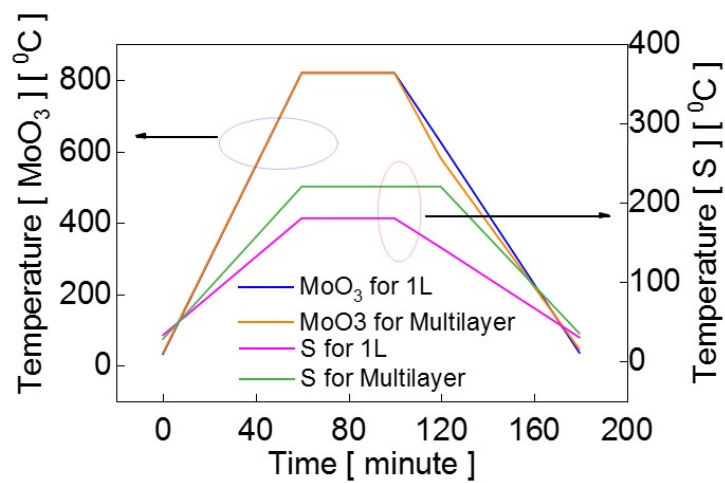

Figure S2 – Programmed temperature profile used for monolayer (1L) and multilayer (ML) MoS<sub>2</sub> film growth.

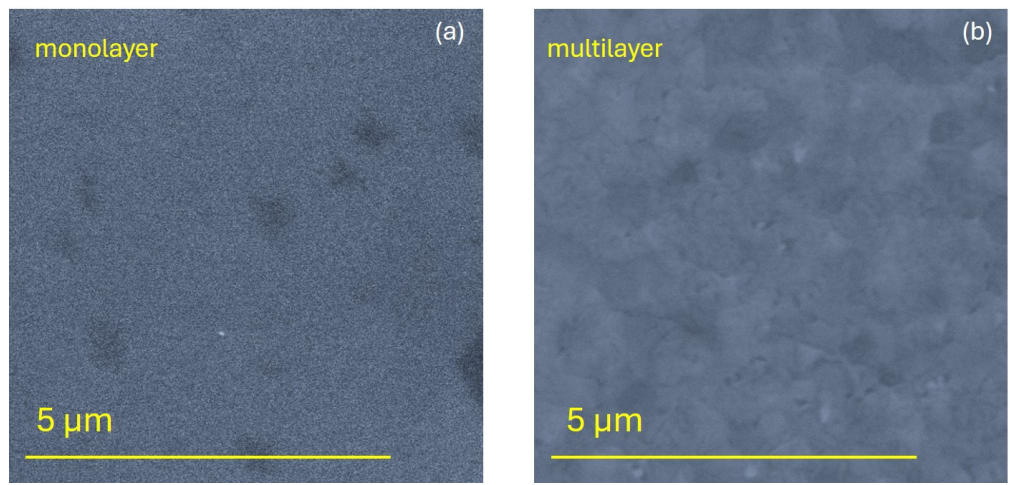

Figure S3 – SEM image of CVD grown (a) 1L-MoS<sub>2</sub> and (b) ML MoS<sub>2</sub> film

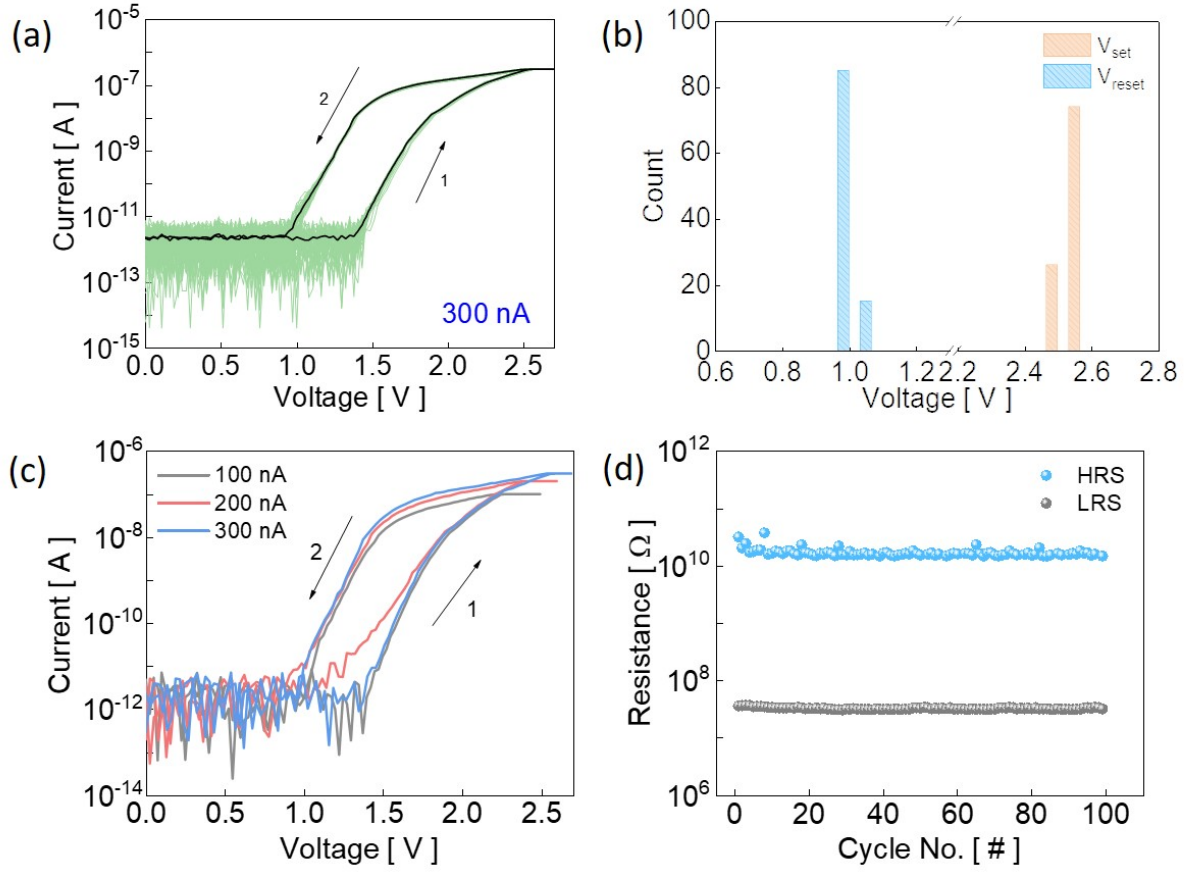

Figure S4 – (a) DC  $I-V$  characteristics for STM device at 300 nA CC and its corresponding, (b) On ( $V_{set}$ ) and Off ( $V_{reset}$ ) state voltage distribution of STM device at 300 nA, (c) DC  $I-V$  measurements at three different current compliances, (d) HRS and LRS state at 300 nA CC (Device area used is  $5 \times 5 \mu\text{m}^2$ ).

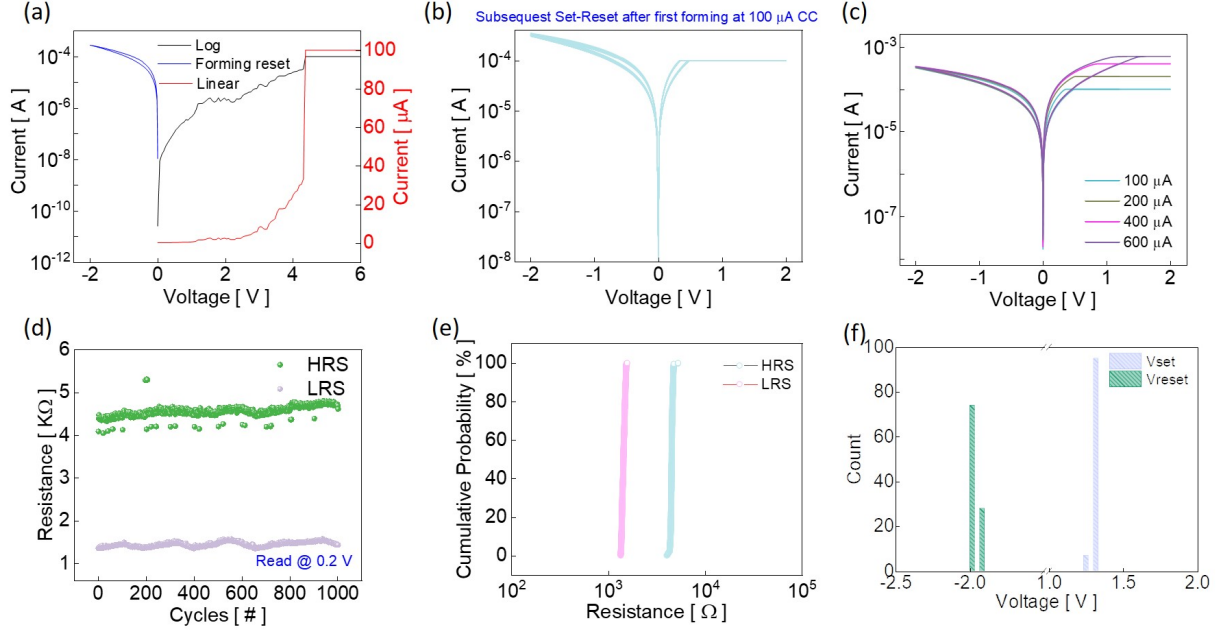

Figure S5 – LTM device (a) Forming step of the ML-MoS<sub>2</sub> device, (b) Subsequent set-reset after first forming at 100  $\mu$ A, (c) DC I-V measurements at four different CC, (d) HRS and LRS state measured at 600  $\mu$ A CC with read voltage 0.2 V, (e) Cumulative probability for HRS and LRS, (f) On ( $V_{set}$ ) and Off ( $V_{reset}$ ) state voltage distributions of LTM device at 600  $\mu$ A (Device area used is  $5 \times 5 \mu\text{m}^2$ ).

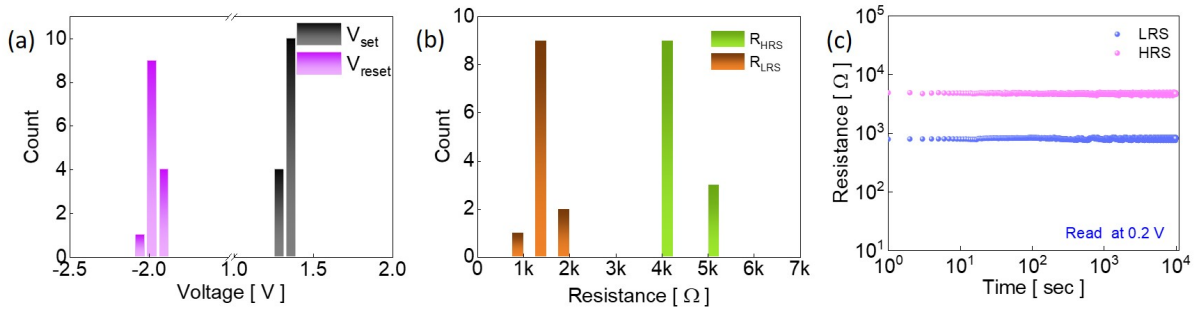

Figure S6 – Device to device variations studied at 600  $\mu$ A over more than 10 different devices on  $5 \times 5 \mu\text{m}^2$  area device for (a)  $V_{Set}$  and  $V_{Reset}$ , (b) HRS and LRS resistances (Read at 0.2 V), (c) Room-temperature retention data studied on a  $25 \mu\text{m}^2$  area device at 600  $\mu$ A current compliance.

Table 1 – Cycle to Cycle and and Device to Device Statistics

| Parameter              | Cycle-Cycle |           | Device-Device |           |
|------------------------|-------------|-----------|---------------|-----------|
|                        | Mean        | Std. Dev. | Mean          | Std. Dev. |
| $R_{on}$ ( $\Omega$ )  | 1.4 k       | 28        | 1.3 k         | 218       |
| $R_{off}$ ( $\Omega$ ) | 4.5 k       | 96        | 4.6 k         | 396       |
| $V_{on}$ (V)           | 1.32        | 0.02      | 1.37          | 0.03      |
| $V_{off}$ (V)          | -1.98       | 0.02      | -1.99         | 0.03      |

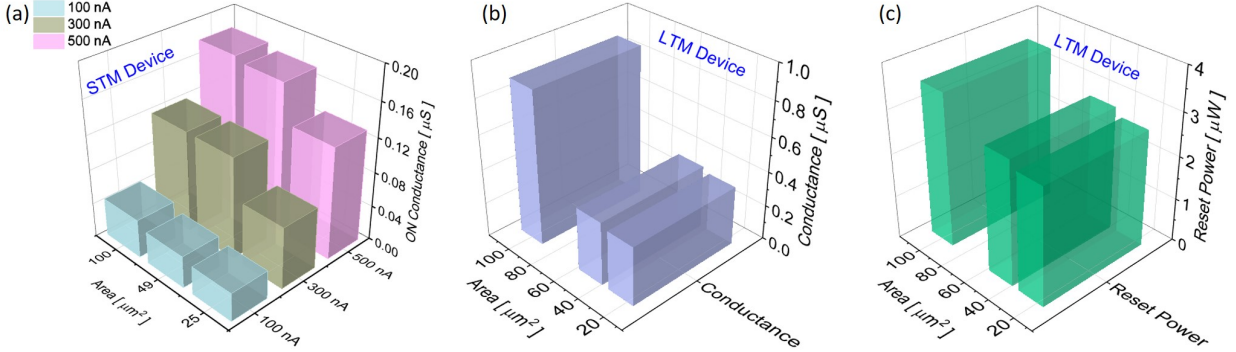

Figure S7 – Area dependent measurements: (a) STM Device - Change in the on-state conductance w.r.t area at different CC values (100 nA, 300 nA, 500 nA). LTM Device: (b) Change in the on- state conductance, and (c) reset power w.r.t area at 100  $\mu$ A CC(data extracted from pulse measurements.)

**NOTE 1:** Figure S11(a) shows one cycle of potentiation (P) operation followed by one cycle of depression (D) operation. Figure S11(b) (top panel) shows the pulse programming scheme for performing potentiation. A sequence of 45 consecutive positive pulses of amplitude 5 V and width of 5  $\mu$ s are used. Similarly, Depression operation uses 45 consecutive negative pulses of amplitude -2 V and width of 5  $\mu$ s, as seen in Figure S11(b) (bottom panel). Figure S11(c) represents multiple cycles of P/D operation, showcasing analog and repeatable conductance tuning using the programming scheme shown in Figure S11(b). C2C fluctuations in conductance tuning of memristive devices are not discussed frequently. To evaluate the cycle-cycle uniformity, we track the conductance of the device after every 25<sup>th</sup> programming pulse (out of a total of 90 pulses) in each P/D cycle. The significance is that 25 consecutive programming pulses tunes the device approximately near the middle of the conductance tuning range. The measured conductance, as a function of the potentiation

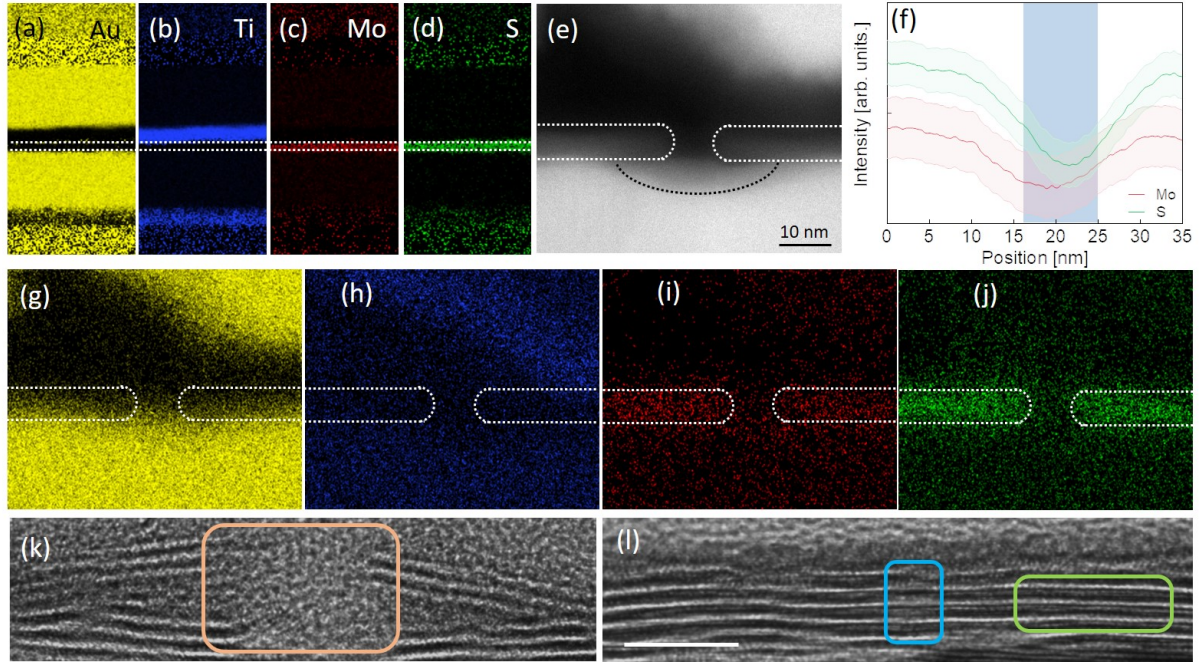

Figure S8 – (a-d) EDS elemental mapping for the elements Au, Ti, Mo, and S, respectively in pristine condition. (e) A high resolution image of the switched device showing the region close to the filament within the device. (f) A line-scan in the switched device indicates generation of S-vacancy in the filamentary region as well as in the bulk of the film. (g-j) Elemental mapping of the region shown in figure (e) for Au, Ti, Mo and S, respectively. Zoomed STEM image of a switched device showing (k) the conductive filament, (l) Zoomed-out image of defects and Au intercalates in MoS<sub>2</sub>, away from the filament region (scale 5 nm).

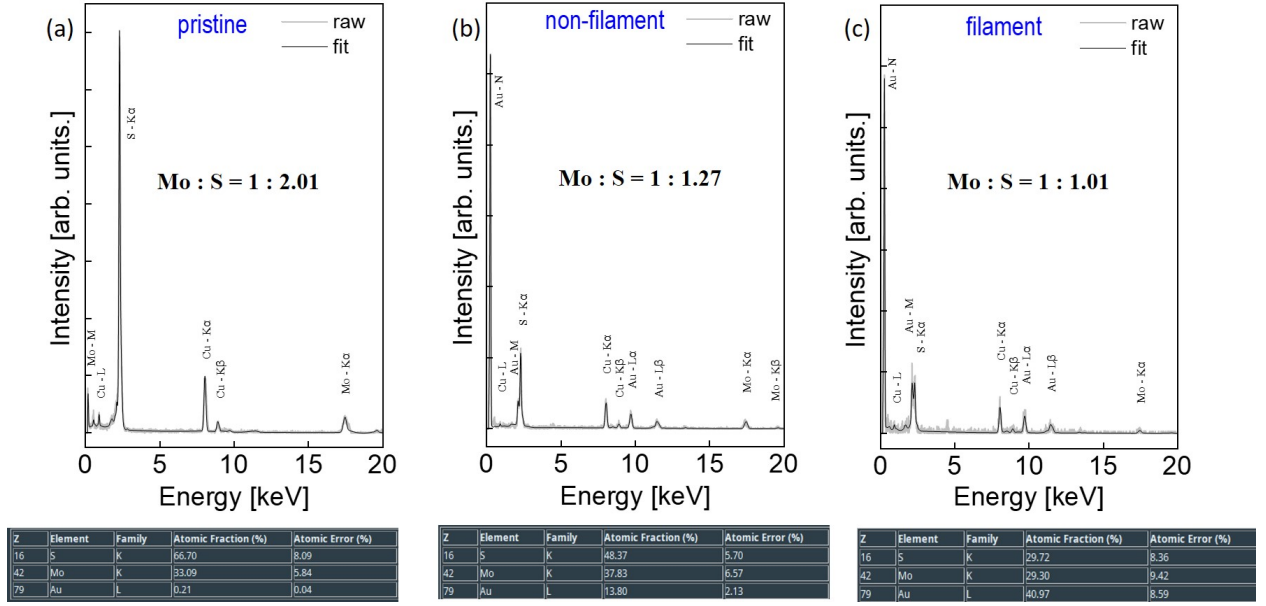

Figure S9 – EDS spectra of the ML-MoS<sub>2</sub> film for (a) a device in the pristine condition, (b) in the non-filamentary region of a switched device, (c) in the filamentary region of a switched device.

cycles is shown in Figure S11(d). The resulting cumulative probability for conductance is plotted in Figure S11(e). We observe a standard error less than 4.6%.

Table 2 – Cycle-to-cycle standard errors in long-term potentiation/depression measurements, evaluated at different programming pulse numbers

| Figure No. | 5 <sup>th</sup> pulse | 35 <sup>th</sup> pulse | 47 <sup>th</sup> pulse | 50 <sup>th</sup> pulse |
|------------|-----------------------|------------------------|------------------------|------------------------|
| S12        | 7.38%                 | 9.20%                  | 1.05%                  | 2.04%                  |

## Note 2: Preprocessing Input:

The Free-Spoken Digit Dataset (FSDD) audio files are first pre-processed to a fixed-length waveform at a sampling rate of 8 kHz. Each waveform is segmented into overlapping short-time frames ( $\approx 25$  ms), followed by a Hamming window. FFT provides the frequency spectrum of each frame, and the spectral energies are passed through a set of triangular filters spaced on the Mel frequency scale, approximating human auditory perception. Logarithmic conversion and discrete cosine transform are applied to produce a set of coefficients. We implement the entire process through librosa. feature.mfcc function, with 13 coefficients

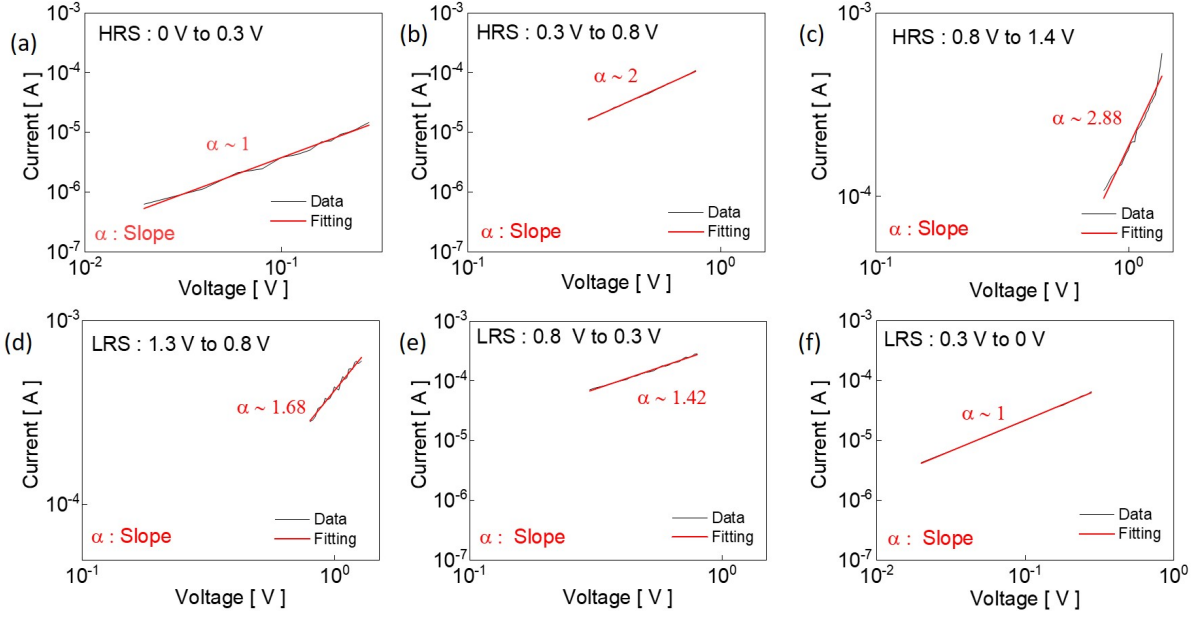

Figure S10 – (a) Double logarithmic plot in HRS showing ohmic conduction at voltages  $< 0.3$  V for slope  $\alpha \approx 1$ , (b) Double logarithmic plot showing SCLC dominated by shallow traps in HRS with a slope  $\alpha \approx 2$ , indicating quadratic relation with the applied voltage up to 0.8 V, (c) Double logarithmic plot showing SCLC in HRS with slope  $\alpha > 2$  where the current follows a higher than quadratic relationship with the applied voltage greater than 0.8 V, (d) Double logarithmic plot showing SCLC in LRS where the current follows a higher with the applied voltage, (e) Double logarithmic plot showing shallow trap SCLC in LRS where the current follows a near-quadratic relation with the applied voltage. (f) Double logarithmic plot showing ohmic conduction in LRS at voltages  $< 0.3$  V for slope  $\alpha \approx 1$ .

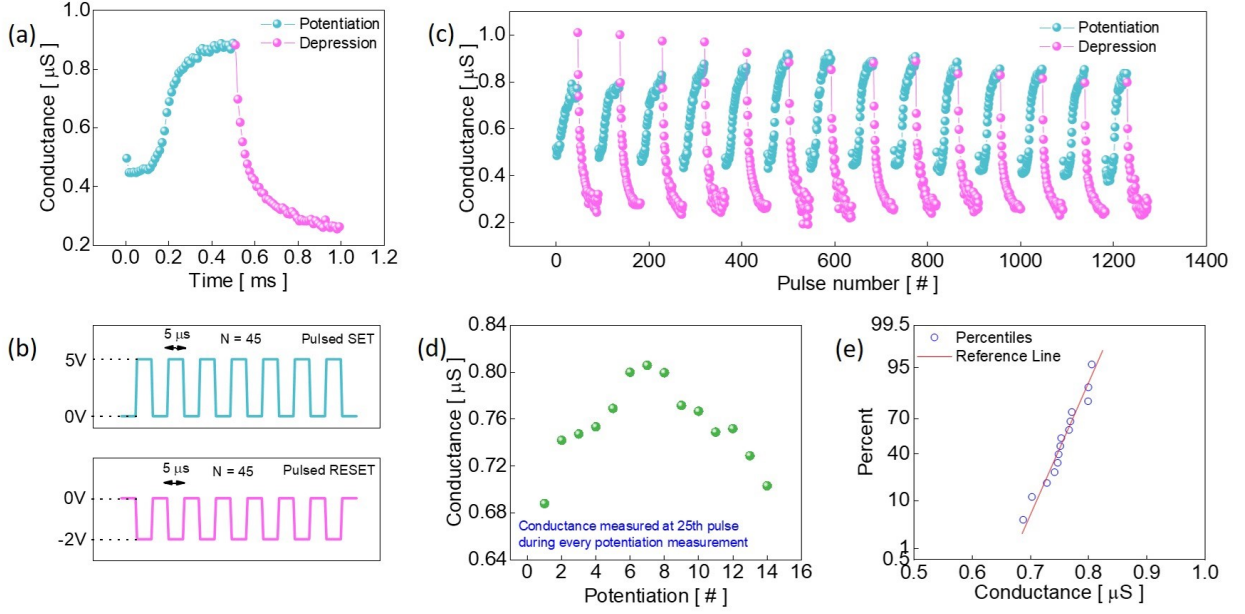

Figure S11 – Analog conductance modulation of individual ML-MoS<sub>2</sub> memristors. (a) One cycle of Potentiation followed by Depression, One Potentiation(Depression) cycle consists of 45 consecutive positive (negative) pulses, (b) Pulsing scheme of each cycle. (c) Write conductance over multiple cycle with respect to pulse number, (d) Device conductance measured at 25<sup>th</sup> pulse out of 45 pulses applied in each potentiation cycle with respect to potentiation cycle number, (e) Cumulative probability of device conductance at 25<sup>th</sup> pulse in each potentiation cycle, (Device area used for measurements is 10  $\mu\text{m} \times 10 \mu\text{m}$ ).

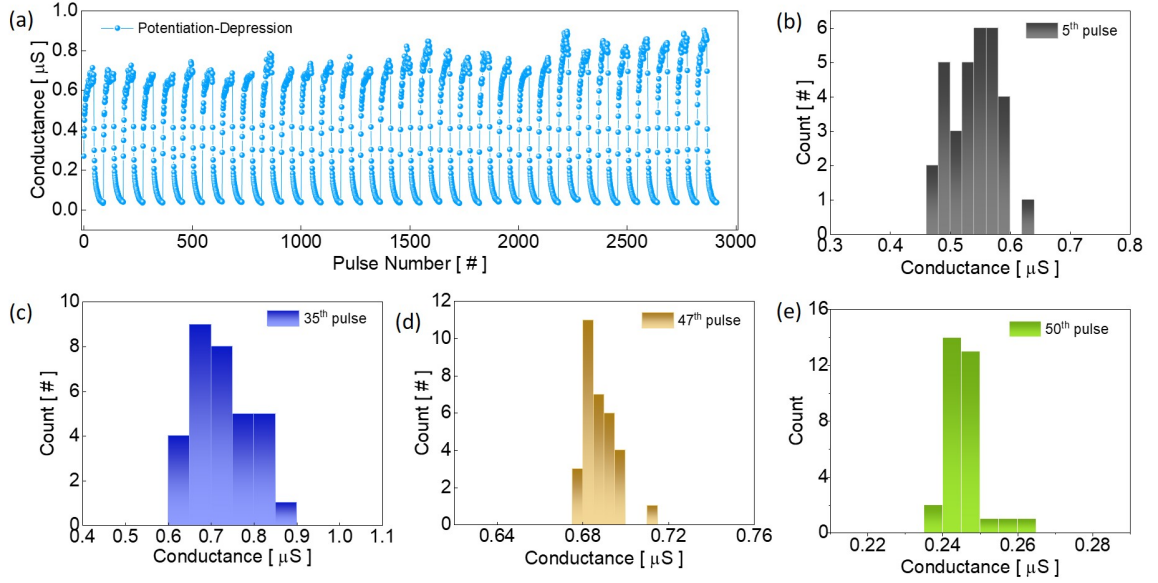

Figure S12 – (a) Potentiation and depression cycles, (b-e) Conductance distribution measured at 5<sup>th</sup>, 35<sup>th</sup>, 47<sup>th</sup>, and 50<sup>th</sup> pulse number of each cycle, (Single cross-point devices with area  $10\text{ }\mu\text{m} \times 10\text{ }\mu\text{m}$ ).

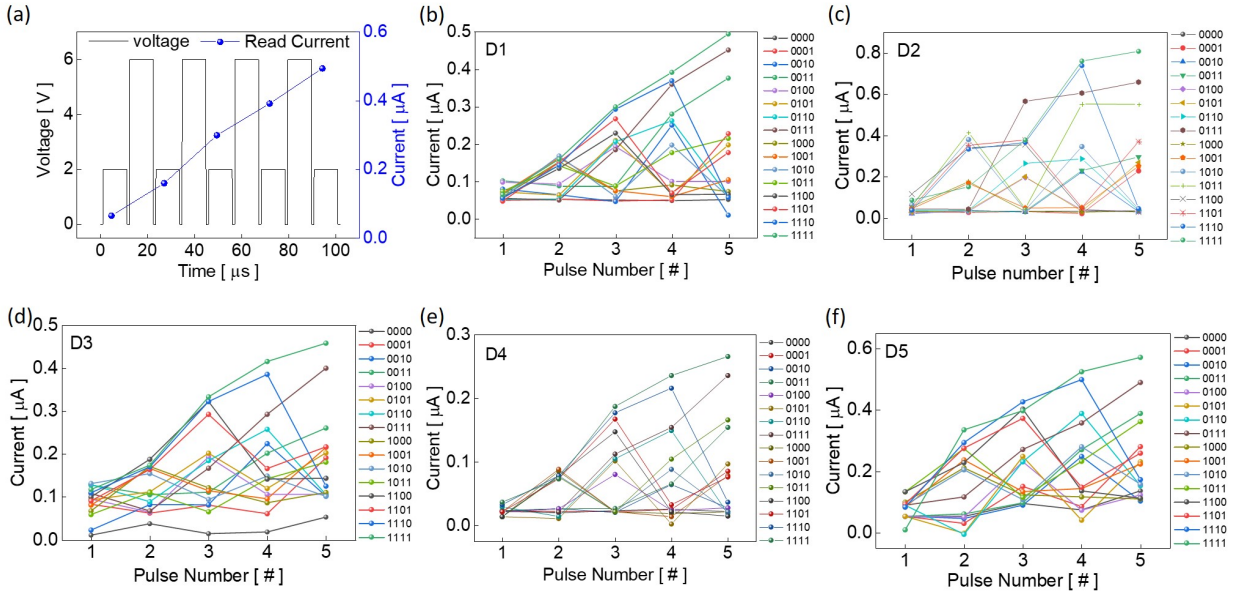

Figure S13 – 16 output states with 4-bit input pulse streams; (a) Voltage and current measured on 4-bit [1111] pulse stream, (b-f) 16 output states extracted from input pulse streams from [0000] to [1111] on five (D1, D2, D3, D4, D5) different devices, (Device area  $7\text{ }\mu\text{m} \times 7\text{ }\mu\text{m}$ ).

retained per frame. The resulting feature matrix has dimensions (frames  $\times$  13), where each row corresponds to one short-time frame of the input speech. Following MFCC extraction, z-score normalization (zero mean, unit variance) is used to standardize the coefficient matrices across the dataset. The above step is performed with the intention of reducing bias from varying speaker intensities and recording conditions. Finally, each feature value is discretized into a 4-bit representation, resulting in binary patterns between 0000 and 1111.

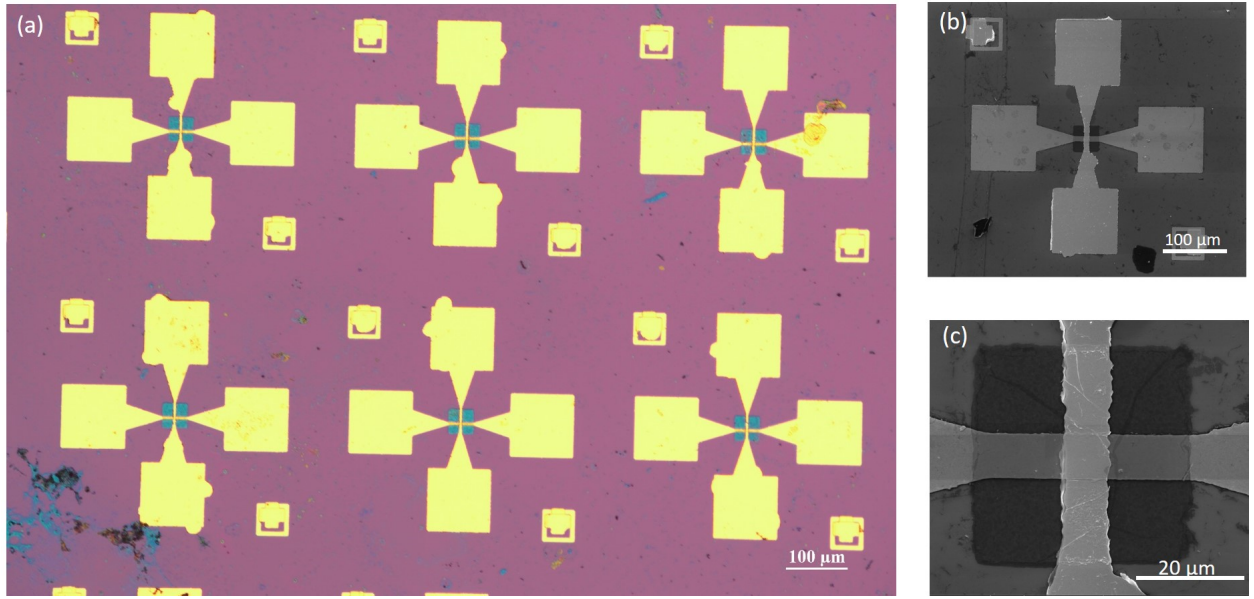

Figure S14 – (a) Optical image of fabricated devices, (b-c) SEM image for the device with area  $10\text{ }\mu\text{m} \times 10\text{ }\mu\text{m}$

## References

- (1) Du, C.; Cai, F.; Zidan, M. A.; Ma, W.; Lee, S. H.; Lu, W. D. Reservoir computing using dynamic memristors for temporal information processing. *Nature communications* **2017**, 8, 2204.
- (2) Mao, J.-Y.; Zheng, Z.; Xiong, Z.-Y.; Huang, P.; Ding, G.-L.; Wang, R.; Wang, Z.-P.; Yang, J.-Q.; Zhou, Y.; Zhai, T.; others Lead-free monocrystalline perovskite resistive switching device for temporal information processing. *Nano Energy* **2020**, 71, 104616.

Table 3 – Summary of memristor-based reservoir computing (RC) systems [R: Recognition, D: Detection, C: Classification]

| Device (C2C)                                                                                                                 | Nodes | Application               | Accuracy (%)   | Power  | WER               |
|------------------------------------------------------------------------------------------------------------------------------|-------|---------------------------|----------------|--------|-------------------|
| Pd/Au/WO <sub>x</sub> /SiO <sub>2</sub> /W <sup>1</sup>                                                                      | 88    | R: MNIST                  | 88.1           | -      | -                 |
| Au/Cs <sub>3</sub> Sb <sub>2</sub> Br <sub>9</sub> /Au (12.57 %) <sup>2</sup>                                                | 5     | R: Letters                | 96             | -      | -                 |
| Ag/Cr/BN/Cr/Ag (26.27 %) <sup>3</sup>                                                                                        | 5     | R: Digits                 | 96             | -      | -                 |
| Ni/WO <sub>x</sub> /ITO (N/A) <sup>4</sup>                                                                                   | 5     | R: Digits                 | 96             | -      | -                 |
| Ag/CsPbI <sub>3</sub> /Ag (12.97 %) <sup>5</sup>                                                                             | 31    | R: neural firing patterns | 87             | 1.2 nW | -                 |
| Au/MAPbI <sub>3</sub> /ITO (N/A) <sup>6</sup>                                                                                | 28    | C: F-MNIST                | 90.1           | -      | -                 |
| Reservoir: Pd/SiO <sub>x</sub> :Ag/Ti/Pt<br>Readout: 1T1R (N/A) <sup>7</sup>                                                 | 110   | R: MNIST                  | 83             | -      | -                 |
| Reservoir: W/HZO/SiO <sub>2</sub> /Si, Readout: Non-volatile RRAM (N/A) <sup>8</sup>                                         | 28    | R: MNIST                  | 96.6           | 35 pW  | -                 |
| Reservoir: Ti/TiOx/Pd, Readout: TiN/TaO <sub>x</sub> /HfAlOy/TiN (N/A) <sup>9</sup>                                          | 24    | D: Arrhythmia             | 96.66          | -      | -                 |
| This Work (Reservoir: MoS <sub>2</sub> based short term device, Readout: MoS <sub>2</sub> based long term device)( $< 4\%$ ) | 8     | R: FSDD                   | $\approx 89.5$ | -      | $\approx 0.2-0.4$ |

- (3) Ding, G.; Chen, R.-S.; Xie, P.; Yang, B.; Shang, G.; Liu, Y.; Gao, L.; Mo, W.-A.; Zhou, K.; Han, S.-T.; others Filament engineering of two-dimensional h-BN for a self-power mechano-nociceptor system. *Small* **2022**, *18*, 2200185.
- (4) Kim, D.; Shin, J.; Kim, S. Implementation of reservoir computing using volatile WO<sub>x</sub>-based memristor. *Applied Surface Science* **2022**, *599*, 153876.
- (5) Zhu, X.; Wang, Q.; Lu, W. D. Memristor networks for real-time neural activity analysis. *Nature communications* **2020**, *11*, 2439.
- (6) Yang, J.; Zhang, F.; Xiao, H.-M.; Wang, Z.-P.; Xie, P.; Feng, Z.; Wang, J.; Mao, J.;

- Zhou, Y.; Han, S.-T. A perovskite memristor with large dynamic space for analog-encoded image recognition. *ACS nano* **2022**, *16*, 21324–21333.
- (7) Midya, R.; Wang, Z.; Asapu, S.; Zhang, X.; Rao, M.; Song, W.; Zhuo, Y.; Upadhyay, N.; Xia, Q.; Yang, J. J. Reservoir computing using diffusive memristors. *Advanced Intelligent Systems* **2019**, *1*, 1900084.
- (8) Yu, J.; Li, Y.; Sun, W.; Zhang, W.; Gao, Z.; Dong, D.; Yu, Z.; Zhao, Y.; Lai, J.; Ding, Q.; others IEEE Symp. on VLSI Tech. 2021.
- (9) Zhong, Y.; Tang, J.; Li, X.; Liang, X.; Liu, Z.; Li, Y.; Xi, Y.; Yao, P.; Hao, Z.; Gao, B.; others A memristor-based analogue reservoir computing system for real-time and power-efficient signal processing. *Nature Electronics* **2022**, *5*, 672–681.
